# Supplementary material for: Global triplewise information trade-off in quantum measurement
Source: arXiv:2104.14078 ancillary file (2021-04-29)
Supplement: Supplementary file 1 [file Supple_RCIBQM_v5.pdf]

# Supplementary Notes for Global triplewise information trade-off in quantum measurement

Seongjin Hong,[1] Yong-Su Kim,[1,2] Young-Wook Cho,[1,3] Jaewan Kim,[4] Seung-Woo Lee,[1,*] and Hyang-Tag Lim[1,2,†]

[1] *Center for Quantum Information, Korea Institute of Science and Technology (KIST), Seoul, 02792, Korea*
[2] *Division of Nano and Information Technology, KIST School, Korea University of Science and Technology, Seoul 02792, Korea*
[3] *Department of Physics, Yonsei University, Seoul 03722, Korea*
[4] *School of Computational Sciences, Korea Institute for Advanced Study, Seoul 02455, Korea*

* swleego@gmail.com
† hyangtag.lim@kist.re.kr

## $F$, $G$, $R$ CALCULATION

To obtain $G$ and $F$, one should perform quantum measurement for a set of nine pure input states known as symmetric and informationally complete positive-operator-valued measures (SIC-POVMs) in qutrit systems [1]. A set of nine states $\{|\nu_i\rangle\}_{i=0}^{8}$ is defined as,

$$|\nu_0\rangle = \frac{1}{\sqrt{2}}\begin{pmatrix}1\\w\\0\end{pmatrix}, |\nu_1\rangle = \frac{1}{\sqrt{2}}\begin{pmatrix}1\\w^2\\0\end{pmatrix}, |\nu_2\rangle = \frac{1}{\sqrt{2}}\begin{pmatrix}1\\w^3\\0\end{pmatrix},$$

$$|\nu_3\rangle = \frac{1}{\sqrt{2}},\begin{pmatrix}0\\1\\w\end{pmatrix} |\nu_4\rangle = \frac{1}{\sqrt{2}}\begin{pmatrix}0\\1\\w^2\end{pmatrix}, |\nu_5\rangle = \frac{1}{\sqrt{2}}\begin{pmatrix}0\\1\\w^3\end{pmatrix},$$

$$|\nu_6\rangle = \frac{1}{\sqrt{2}}\begin{pmatrix}w\\0\\1\end{pmatrix}, |\nu_7\rangle = \frac{1}{\sqrt{2}}\begin{pmatrix}w^2\\0\\1\end{pmatrix}, |\nu_8\rangle = \frac{1}{\sqrt{2}}\begin{pmatrix}w^3\\0\\1\end{pmatrix},$$

where $w = e^{2i\pi/3}$ is the relative phase between two basis. We measure the outcomes for $\{|\nu_i\rangle\}_{i=0}^{8}$ for a given set of measurement operators $\hat{M}_r$, which satisfying the completeness relation $\sum_r \hat{M}_r^\dagger \hat{M}_r = \hat{I}$ with possible outcomes $r = 0, ..., N$, then $G$ and $F$ can be calculated by averaging the outcomes as,

$$\begin{aligned} G &= \int d\psi \sum_{r=0}^{N} \langle\psi|\hat{M}_r^\dagger \hat{M}_r|\psi\rangle |\langle\psi|\widetilde{\psi}_r\rangle|^2 \\ &= \sum_{j=0}^{8}(\sum_{r=0}^{N}\langle\nu_j|\hat{M}_r^\dagger \hat{M}_r|\nu_j\rangle|\langle\nu_j|\widetilde{\psi}_r\rangle|^2). \end{aligned} \tag{1}$$

Here, we take the optimal guessing strategy, where $|\widetilde{\psi}_r\rangle = |r\rangle$ with $r = 0, 1, 2$ for the outcome $r$.

$$F = \int d\psi \sum_{r=0}^{N} |\langle\psi|\hat{M}_r|\psi\rangle|^2 = \frac{1}{9}\sum_{j=0}^{8}\sum_{r=0}^{N} Tr[\rho_j \cdot \rho_{r,j}], \tag{2}$$

where $\rho_j = |\nu_j\rangle\langle\nu_j|$ and $\rho_{j,r} = \hat{M}_r^\dagger \hat{M}_r |\nu_j\rangle\langle\nu_j|$. The reversing operator $\hat{R}^r$ is defined as $\hat{R}^r \hat{M}_r|\psi\rangle = \eta_r|\psi\rangle$. Here, $\eta_r$ is a nonzero complex variable, and $|\eta_r|^2$ is the success probability of the reversing operation. $R$ is then calculated by

$$R = \sum_{r=0}^{N}|\eta_r|^2 = \sum_{r=0}^{N}\frac{|\langle\psi|\hat{R}^{r\dagger}\hat{M}_r^\dagger \hat{R}_r \hat{M}_r|\psi\rangle|^2}{|\langle\psi|\psi\rangle|^2}, \tag{3}$$

where we choose $|\psi\rangle = |\nu_2\rangle$.

## EXPERIMENTAL DETAILS

### A. State preparation and measurement.

As described in the main text, we can prepare an arbitrary qutrit state $|\psi\rangle = a_0|0\rangle + e^{i\phi_1}a_1|1\rangle + e^{i\phi_2}a_2|2\rangle$ with our experimental set up as shown in Supplementary Figure 1. Here, in order to obtain $G$, $F$, and $R$, it is necessary to measure the outcomes for a set of nine pure states $\{|\nu_i\rangle\}_{i=0}^{8}$ [1]. The half-wave plate (HWP) angles used for implementing SIC-POVM basis are shown in Supplementary Table I. For a state preparation as shown in Supplementary Table I, the mode-amplitude $a_i$ $(i = 0, 1, 2)$ is varied by $H_A$ and $H_B$, and the relative phases $\phi_i$ with $i = 1, 2$ are implemented by the HWP angle $\alpha_i$ between two quarter-wave plates (QWPs) at 45°. For the measurement, the mode-amplitude is varied by $H_C$ and $H_D$ and HWP angle $\beta_i$ are used for adjusting relative phases. In order to confirm that the input state and the measurement basis are well prepared as $\{|\nu_i\rangle\}_{i=0}^{8}$, we investigate the encoded phase shift

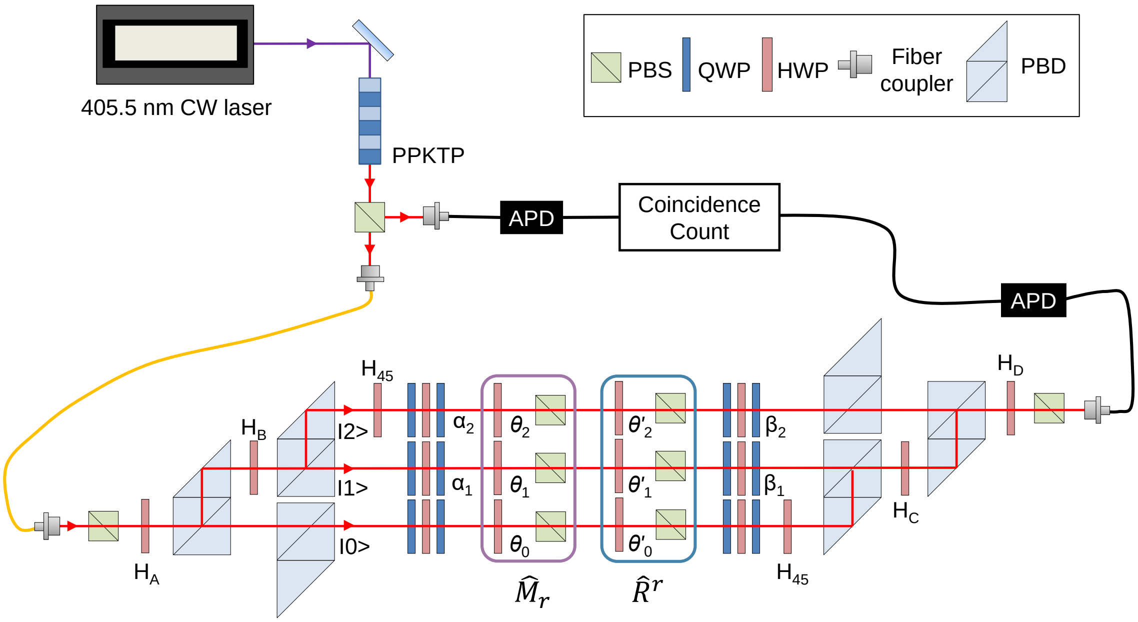


Supplementary Figure 1. Experimental setup. PBD: Polarizing beam displacer, PBS: Polarizing beam splitter, QWP: Quarter-wave plate, HWP: Half-wave plate, APD: Avalanche photo diode, PPKTP: periodically poled $KTiOPO_4$.

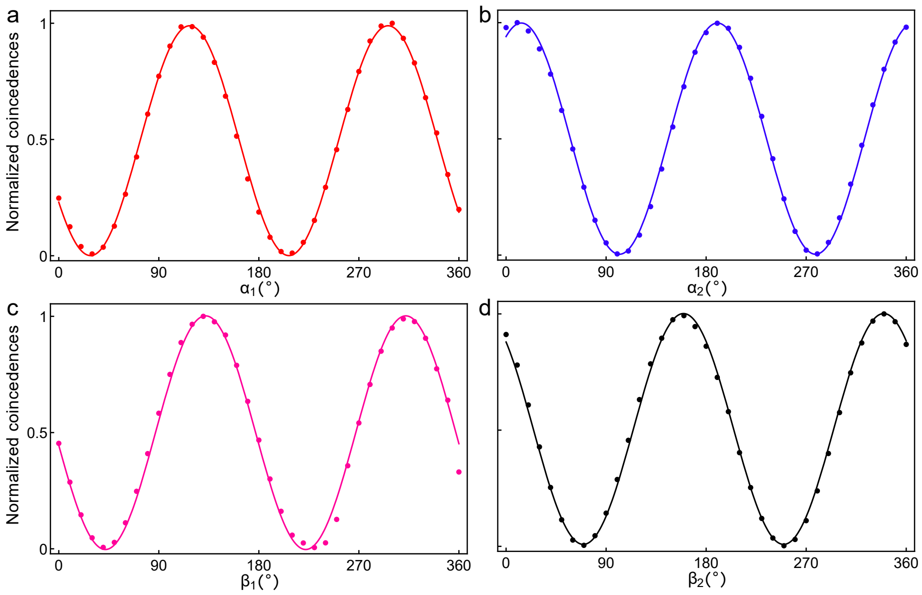


Supplementary Figure 2. Coincidence counts for an input state $|\nu_0\rangle$ with measurement $|\nu_0\rangle\langle\nu_0|$ depending on (a) $\phi_1 = 2\alpha_1$ and (c) $\phi_1 = 2\beta_1$. Coincidence counts for an input state $|\nu_6\rangle$ with measurement $|\nu_6\rangle\langle\nu_6|$ depending on (b) $\phi_2 = 2\alpha_2$ and (d) $\phi_2 = 2\beta_2$. Here $\phi_i = 2\alpha_i$ and $\phi_i = 2\beta_i$ are depending on state generation and measurement, respectively. All visibility values are higher than 0.99

$\phi_i = 2\alpha_i$ ($\phi_i = 2\beta_i$) depending on $\alpha_i$ and $\beta_i$. First, we set the input state as $|\nu_0\rangle$ and measurement set as $|\nu_0\rangle\langle\nu_0|$, and we measure the coincidence as a function of $\phi_1$ depending on $\alpha_1$ and $\beta_1$, respectively. Also we set the input state as $|\nu_6\rangle$ and measurement set as $|\nu_6\rangle\langle\nu_6|$, and we measure the coincidence as a function of $\phi_2$ depending on $\alpha_2$ and $\beta_2$, respectively. The results are fitted with sinusoidal function, and they show that the relation between the relative phase and the angle of HWP is well matched with $\phi = 2\alpha$ ($\phi = 2\beta$) as shown in Supplementary Figure 2. We attribute the experimental errors with respect to the theoretical prediction to both a non-unity visibility of the measured interference and imperfect alignment of our experimental setup.

| Input state | $H_A$ | $H_B$ | $\alpha_1$ | $\alpha_2$ | Measurement | $H_C$ | $H_D$ | $\beta_1$ | $\beta_2$ |
|---|---|---|---|---|---|---|---|---|---|
| $\|\nu_0\rangle$ | 22.5° | 45° | 60° | 0° | $\|\nu_0\rangle\langle\nu_0\|$ | 22.5° | 45° | 60° | 0° |
| $\|\nu_1\rangle$ | 22.5° | 45° | 120° | 0° | $\|\nu_1\rangle\langle\nu_1\|$ | 22.5° | 45° | 120° | 0° |
| $\|\nu_2\rangle$ | 22.5° | 45° | 0° | 0° | $\|\nu_2\rangle\langle\nu_2\|$ | 22.5° | 45° | 0° | 0° |
| $\|\nu_3\rangle$ | 45° | 22.5° | 0° | 60° | $\|\nu_3\rangle\langle\nu_3\|$ | 45° | 22.5° | 0° | 60° |
| $\|\nu_4\rangle$ | 45° | 22.5° | 0° | 120° | $\|\nu_4\rangle\langle\nu_4\|$ | 45° | 22.5° | 0° | 120° |
| $\|\nu_5\rangle$ | 45° | 22.5° | 0° | 0° | $\|\nu_5\rangle\langle\nu_5\|$ | 45° | 22.5° | 0° | 0° |
| $\|\nu_6\rangle$ | 22.5° | 0° | 0° | −60° | $\|\nu_6\rangle\langle\nu_6\|$ | 0° | 22.5° | 0° | −60° |
| $\|\nu_7\rangle$ | 22.5° | 0° | 0° | −120° | $\|\nu_7\rangle\langle\nu_7\|$ | 0° | 22.5° | 0° | −120° |
| $\|\nu_8\rangle$ | 22.5° | 0° | 0° | 0° | $\|\nu_8\rangle\langle\nu_8\|$ | 0° | 22.5° | 0° | 0° |

Supplementary Table I. HWP angle settings for state preparation and measurement

| $\hat{M}_0^{(0)}$ | | | | | $\hat{R}^0$ | | |
|---|---|---|---|---|---|---|---|
| $p$ | $\theta_0(^\circ)$ | $\theta_1(^\circ)$ | $\theta_2(^\circ)$ | $p$ | $\theta'_0(^\circ)$ | $\theta'_1(^\circ)$ | $\theta'_2(^\circ)$ |
| 0.333 | 0 | 0 | 0 | | 0 | 0 | 0 |
| 0.5 | 22.5 | 30 | 30 | | 22.5 | 0 | 0 |
| 0.65 | 18.1 | 32.6 | 32.6 | | 29.4 | 0 | 0 |
| 0.8 | 13.3 | 35.8 | 35.8 | | 34.7 | 0 | 0 |
| 0.95 | 6.5 | 40.5 | 40.5 | | 40.3 | 0 | 0 |
| 1 | 0 | 45 | 45 | | 45 | 0 | 0 |

Supplementary Table II. HWP angle settings for $\hat{M}_0^{(0)}$ and corresponding $\hat{R}^0$ for various $p$.

### B. POVM setting

POVMs for a general quantum measurement $\hat{M}_r$ and a reversing measurement $\hat{R}^r$ are realized with a set of HWPs and polarizing beam splitters (PBSs). Since a PBS transmits (reflects) the horizontally (vertically) polarized photons, by adjusting the angle of HWP before a PBS we can set the transmission ratio for photons passing through a PBS. Using a set of a HWP and a PBS, a generalized quantum measurement operator is then given as $\hat{M}_r = \lambda_0^r|0\rangle\langle 0| + \lambda_1^r|1\rangle\langle 1| + \lambda_2^r|2\rangle\langle 2|$. The strength of the generalized quantum measurement $\lambda_i^r$ is set by angles of HWP $\theta$ as $\lambda_i^r = \cos 2\theta_i$ for $i = 0, 1, 2$. Its reversing operator can be realized by the same way as a generalized quantum measurement operator. Note that our scheme can provide a continuous measurement strength of $0 \le \lambda_i^r \le 1$, which shows clear advantages compared to the previous implementation reported in Ref. [2]. For example, to implement a generalized quantum measurement operation $\hat{M}_0^{(0)} = \sqrt{p}|0\rangle\langle 0| + \sqrt{(1-p)/2}(|1\rangle\langle 1| + |2\rangle\langle 2|)$ for $p = 1, 0.95, 0.8, 0.65, 0.5, 0.333$, the HWP angle set for $\hat{M}_0^{(0)}$ are determined as shown in Supplementary Table II. The HWP angle settings for its reversing operator $\hat{R}^0$ corresponding $\hat{M}_0$ is also provided in Supplementary Table II.

### C. Explicit forms of different types of quantum measurement $\hat{M}_r^{(t)}$

The explicit forms of different types of quantum measurement $\hat{M}_r^{(t)}$ are described in Supplementary Table III with $t = 0, 1, 2, 3, 4$.

### D. Information contents of $G$, $F$, $R$ depending on measurement parameter $p$

The obtained results of information contents $G$, $F$, and $R$ for each $\hat{M}_r^{(t)}$ with $t = 0, 1, 2, 3, 4$ with respect to the measurement parameter $p$ are shown in Supplementary Figure 3.

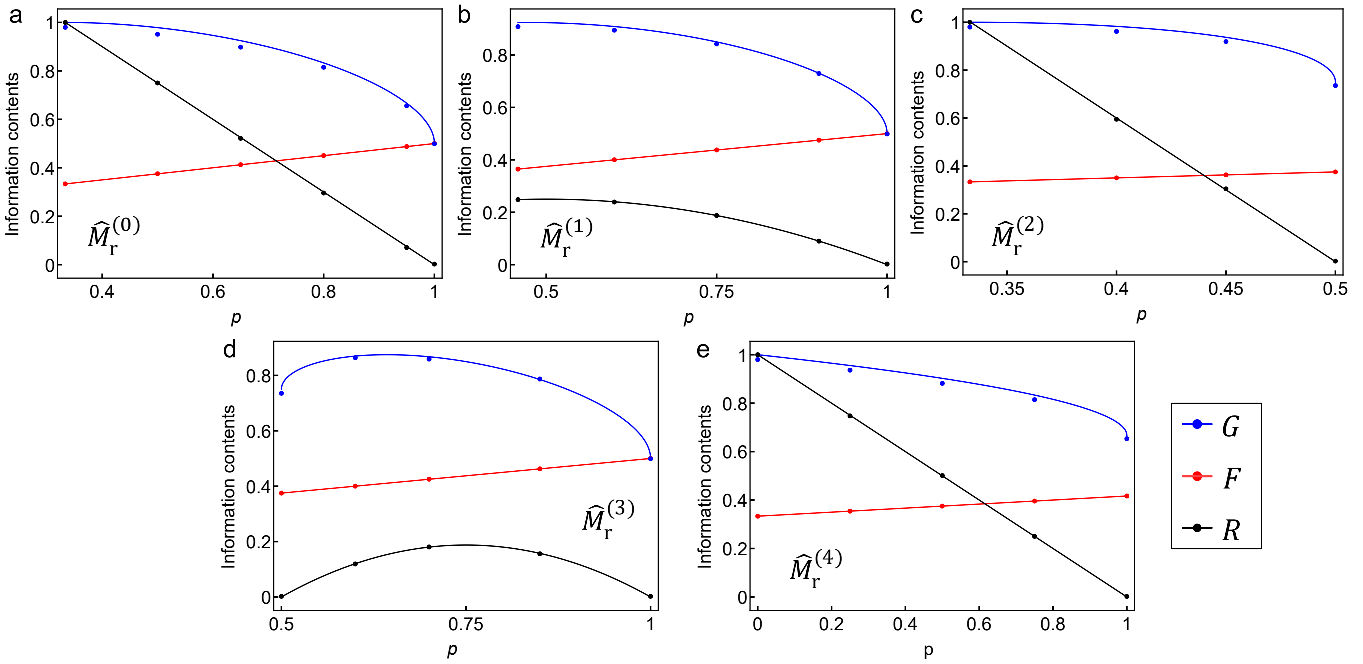


Supplementary Figure 3. Information contents ($G$, $F$, $R$) for quantum measurements depending on measurement parameter $p$. The experimentally obtained $G$, $F$, and $R$ for each $\hat{M}_r^{(t)}$ with respect to $p$ is plotted as a dot and the solid lines represent the ideal relations between the information contents and $p$.

TABLE III. The measurement strength for different types of quantum measurement $\hat{M}_r^{(t)}$

| | $\lambda_0^r$ | $\lambda_1^r$ | $\lambda_2^r$ | $p$ range |
|---|---|---|---|---|
| $\hat{M}_0^{(0)}$ | $\sqrt{p}$ | $\sqrt{\frac{1-p}{2}}$ | $\sqrt{\frac{1-p}{2}}$ | $1/3 \leq p \leq 1$ |
| $\hat{M}_1^{(0)}$ | $\sqrt{\frac{1-p}{2}}$ | $\sqrt{p}$ | $\sqrt{\frac{1-p}{2}}$ | $1/3 \leq p \leq 1$ |
| $\hat{M}_2^{(0)}$ | $\sqrt{\frac{1-p}{2}}$ | $\sqrt{\frac{1-p}{2}}$ | $\sqrt{p}$ | $1/3 \leq p \leq 1$ |
| $\hat{M}_0^{(1)}$ | $\sqrt{p}$ | $\sqrt{(1-p)(3-p)}$ | $\sqrt{p(1-p)}$ | $0.4586 \leq p \leq 1$ |
| $\hat{M}_1^{(1)}$ | $\sqrt{p(1-p)}$ | $\sqrt{p}$ | $\sqrt{(1-p)(3-p)}$ | $0.4586 \leq p \leq 1$ |
| $\hat{M}_2^{(1)}$ | $\sqrt{(1-p)(3-p)}$ | $\sqrt{p(1-p)}$ | $\sqrt{p}$ | $0.4586 \leq p \leq 1$ |
| $\hat{M}_0^{(2)}$ | $\sqrt{p}$ | $\sqrt{p}$ | $\sqrt{1-2p}$ | $1/3 \leq p \leq 1/2$ |
| $\hat{M}_1^{(2)}$ | $\sqrt{1-2p}$ | $\sqrt{p}$ | $\sqrt{p}$ | $1/3 \leq p \leq 1/2$ |
| $\hat{M}_2^{(2)}$ | $\sqrt{p}$ | $\sqrt{1-2p}$ | $\sqrt{p}$ | $1/3 \leq p \leq 1/2$ |
| $\hat{M}_0^{(3)}$ | $\sqrt{p}$ | $\sqrt{p^2-\frac{5}{2}p+\frac{3}{2}}$ | $\sqrt{-p^2+\frac{3}{2}p-\frac{1}{2}}$ | $1/2 \leq p \leq 1$ |
| $\hat{M}_1^{(3)}$ | $\sqrt{-p^2+\frac{3}{2}p-\frac{1}{2}}$ | $\sqrt{p}$ | $\sqrt{p^2-\frac{5}{2}p+\frac{3}{2}}$ | $1/2 \leq p \leq 1$ |
| $\hat{M}_2^{(3)}$ | $\sqrt{p^2-\frac{5}{2}p+\frac{3}{2}}$ | $\sqrt{-p^2+\frac{3}{2}p-\frac{1}{2}}$ | $\sqrt{p}$ | $1/2 \leq p \leq 1$ |
| $\hat{M}_0^{(4)}$ | 1 | $\sqrt{1-p}$ | 1 | $0 \leq p \leq 1$ |
| $\hat{M}_1^{(4)}$ | 0 | $\sqrt{p}$ | 0 | $0 \leq p \leq 1$ |

### E. Pairwise trade-off relations for a non-optimal measurement $\hat{M}_r^{(4)}$

A non-optimal quantum measurement $\hat{M}_r^{(4)}$ is defined by $\hat{M}_0^{(4)} = |0\rangle\langle 0| + \sqrt{1-p}|1\rangle\langle 1| + |2\rangle\langle 2|$ and $\hat{M}_1^{(4)} = \sqrt{p}|1\rangle\langle 1|$ with $0 \leq p \leq 1$. We experimentally obtain $G$, $F$, and $R$ by changing $p$ and the pairwise trade-off relations are plotted in Supplementary Figure 4. As shown in Supplementary Figure 4, we can find that any of the trade-off relations is

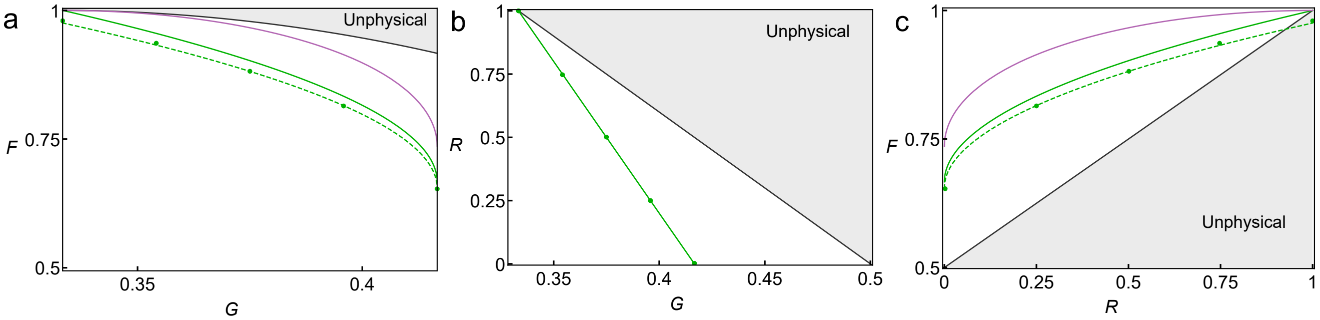


Supplementary Figure 4. Experimentally obtained pairwise trade-off relations for $G$-$F$ (**a**), $G$-$R$ (**b**), and $F$-$R$ (**c**). Experimental results are represented by dots, where the green solid lines indicate the ideal trade-off relations, and the dashed lines represent the fitted trade-off relations assuming a non-ideal input state with $e = 0.963$. The purple solid line represents the global trade-off relation for $\hat{M}_r^{(4)}$.

not saturated except when it corresponds to a unitary operation ($p = 0$).

### F. Quantum process tomography

Quantum process tomography allows us to experimentally reconstruct an unknown quantum operation. In a qutrit system, a quantum operation $\varepsilon(\rho_{in})$ can be represented by $\varepsilon(\rho_{in}) = \sum_{m,n=0}^{8} \chi_{m,n}\Lambda_m\rho_{\rm in}\Lambda_n^\dagger$ where $\{\Lambda_m\}_{m=0}^{8}$ is a complete set of $3 \times 3$ dimensional operator basis. Then, the $\chi$ matrix can completely characterize the quantum operation. In this work, we chose the complete operator basis set consisting of nine operators $\{\Lambda_m\}_{m=0}^{8}$ as follow [1],

$$\Lambda_0 = \begin{pmatrix}1 & 0 & 0\\ 0 & 1 & 0\\ 0 & 0 & 1\end{pmatrix}, \Lambda_1 = \begin{pmatrix}0 & 1 & 0\\ 1 & 0 & 0\\ 0 & 0 & 0\end{pmatrix}, \Lambda_2 = \begin{pmatrix}0 & -i & 0\\ i & 0 & 0\\ 0 & 0 & 0\end{pmatrix},$$

$$\Lambda_3 = \begin{pmatrix}1 & 0 & 0\\ 0 & -1 & 0\\ 0 & 0 & 0\end{pmatrix}, \Lambda_4 = \begin{pmatrix}0 & 0 & 1\\ 0 & 0 & 0\\ 1 & 0 & 0\end{pmatrix}, \Lambda_5 = \begin{pmatrix}0 & 0 & -i\\ 0 & 0 & 0\\ i & 0 & 0\end{pmatrix},$$

$$\Lambda_6 = \begin{pmatrix}0 & 0 & 0\\ 0 & 0 & 1\\ 0 & 1 & 0\end{pmatrix}, \Lambda_7 = \begin{pmatrix}0 & 0 & 0\\ 0 & 0 & -i\\ 0 & i & 0\end{pmatrix}, \Lambda_8 = \frac{1}{\sqrt{3}}\begin{pmatrix}1 & 0 & 0\\ 0 & 1 & 0\\ 0 & 0 & -2\end{pmatrix}.$$

The $\chi$ matrices for $\hat{R}^r\hat{M}_r$ is experimentally reconstructed with nine SIC-POVM input states $\{|\nu_i\rangle\}_{i=0}^{8}$ using a maximum-likelihood estimation process. Since the reversing operation $\hat{R}^r$ can probabilistically recover the initial quantum state, the quantum operation of $\hat{R}^r\hat{M}_r$ corresponds to an identity operation $\hat{I} = \Lambda_0$. The experimentally reconstructed QPT matrix $\chi_{\rm exp}$ for $\hat{R}^1\hat{M}_1^{(4)}$ with $p = 0.5$ is shown in Supplementary Figure 5. Furthermore, to quantify the quality of $\hat{R}^r\hat{M}_r$ operation, we calculate the process fidelity $F_\chi$ =Tr$[\chi_{\rm exp}\chi_{\rm ideal}]$, which defined as the overlap between $\chi_{\rm exp}$ and ideal matrix $\chi_{\rm ideal} = \hat{I}$. The experimentally obtained $F_\chi$ values for various POVM sets are provided in Supplementary Table IV.

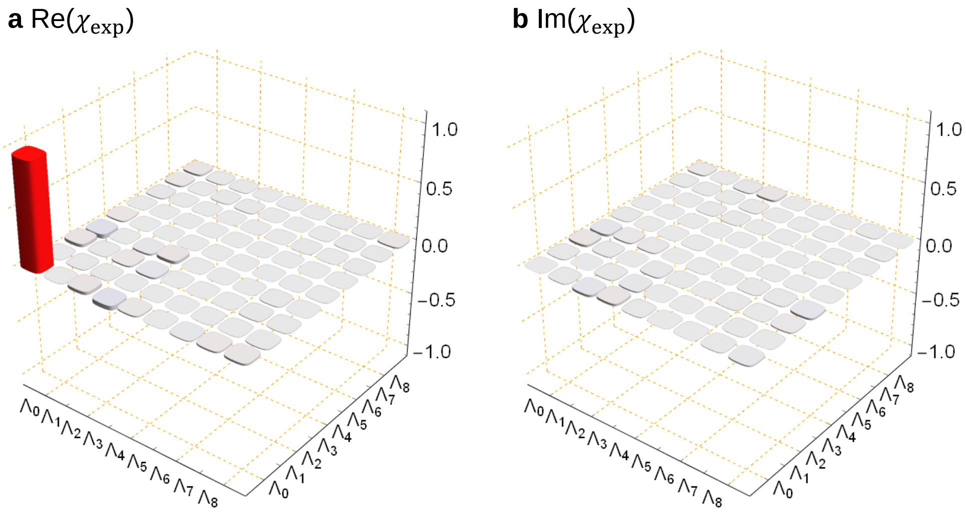


Supplementary Figure 5. Experimentally reconstructed process matrix $\chi_{\rm exp}$ for $\hat{R}^1\hat{M}_1^{(4)}$ with $p = 0.5$.

| | $p$ | $F_\chi(r=0)$ | $F_\chi(r=1)$ | $F_\chi(r=2)$ |
|---|---|---|---|---|
| $\hat{M}_r^{(0)}$ | 0.33 | $0.968 \pm 0.001$ | − | − |
| $\hat{M}_r^{(1)}$ | 0.46 | $0.914 \pm 0.002$ | $0.906 \pm 0.003$ | $0.905 \pm 0.003$ |
| $\hat{M}_r^{(2)}$ | 0.45 | $0.931 \pm 0.002$ | $0.929 \pm 0.002$ | $0.93 \pm 0.002$ |
| $\hat{M}_r^{(3)}$ | 0.7 | $0.907 \pm 0.002$ | $0.908 \pm 0.003$ | $0.91 \pm 0.003$ |
| $\hat{M}_r^{(4)}$ | 0.5 | $0.943 \pm 0.002$ | $0.945 \pm 0.002$ | − |

Supplementary Table IV. Process fidelity $F_\chi$ of various $\hat{R}^r\hat{M}_r$ operations with a particular measurement strength $p$. The errors correspond to one standard deviation and are obtained by performing 100 Monte-Carlo simulation runs by taking into account of the Poissonian photon counting statics.

[1] Lim, H. T., Kim, Y. S., Ra, Y. S., Bae, J., & Kim, Y. H. Experimental realization of an approximate transpose operation for qutrit systems using a structural physical approximation. *Phys. Rev. A* **86**, 042334 (2012).

[2] Lim, H. T., Ra, Y. S., Hong, K. H., Lee, S. W., & Kim, Y. H.Fundamental bounds in measurements for estimating quantum states. *Phys. Rev. Lett.* **113**, 020504 (2014).
